# Supplementary material for: Crossover from quasi-static to dense flow regime in compressed frictional granular media
Source: arXiv:1208.1930 source file (2013-05-15)
Supplement: Supplementary file 1 [file SuppMat.pdf]

# Crossover from quasi-static to dense flow regime in compressed frictional granular media.

Florent Gimbert, David Amitrano and Jérôme Weiss

## 1 Determination of the travel time of an elastic wave through the granular sample

Figure S1 shows a typical macroscopic stress versus strain curve obtained when loading a granular sample of 10000 grains by setting the axial stress increment to $\delta\sigma_1 = 1.10^{-7}\sigma_3$, i.e. imposing a loading rate that is 10 times smaller than the one considered in the main text. In this configuration, local plastic instabilities associated to a local flatness of the stress-versus strain curve are very brutal and are followed by sample oscillations, observed immediately after these plastic instabilities. These oscillations are expected to result from sudden stress redistributions following large plastic events and can here be observed only because of the very slow loading conditions considered. In the main text, a compromise in the loading rate is done choosing a value of $\delta\sigma_1 = 1.10^{-6}\sigma_3$, i.e. large enough to limit these elastic sample oscillations and small enough in order to remain in the quasi-static regime (see section 4).

Figure S2 shows typical horizontal displacements of regularly selected grains along a vertical profile during one of these time periods of oscillations. Similar observations can be done considering the vertical displacements of grains selected along an horizontal profile. A stationary wave, that exhibits a spatial period $\lambda = L_s$, where $L_s$ is the square root of the sample area, can easily be identified on these snapshots. As $c = \lambda/T$, where $c$ is the wave velocity and $T$ is the time period of oscillations, we can write

$$T = L_s/c. \tag{1}$$

and $T$ also corresponds to the travel time of the elastic wave through the granular assembly. The value of $T$ can be accurately identified by performing the Fourier transform of the radial deformation $\epsilon_2$ (Figure S3). At various sample sizes, i.e. using $N_g = 2500$, $N_g = 10000$ and $N_g = 44944$, a clear peak associated to the characteristic frequency $f_{N_g} = 1/T_{N_g}$ of the oscillation mode is reported on the fourier transorm. The collapse analysis shows that the frequency depends linearly on the sample size, as expected for a travelling elastic wave, and that $T_{N_g}$ can be approximated by

$$T_{N_g} = \sqrt{N_g} \times 100 \times t_r \tag{2}$$

where $t_r$ is the discretisation time interval.

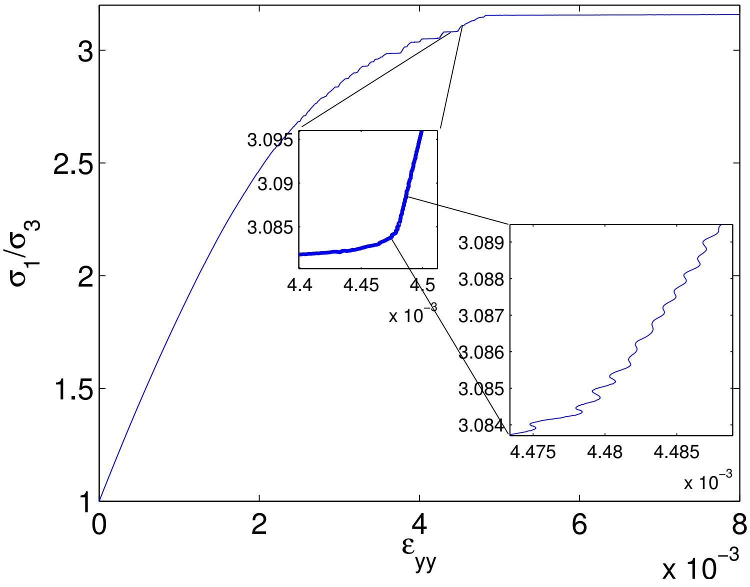


Figure 1: Exemple of an oscillation on the stress-strain curve. The stress increment imposed at each time step is equal to $1.10^{-7} \times \sigma_3$.

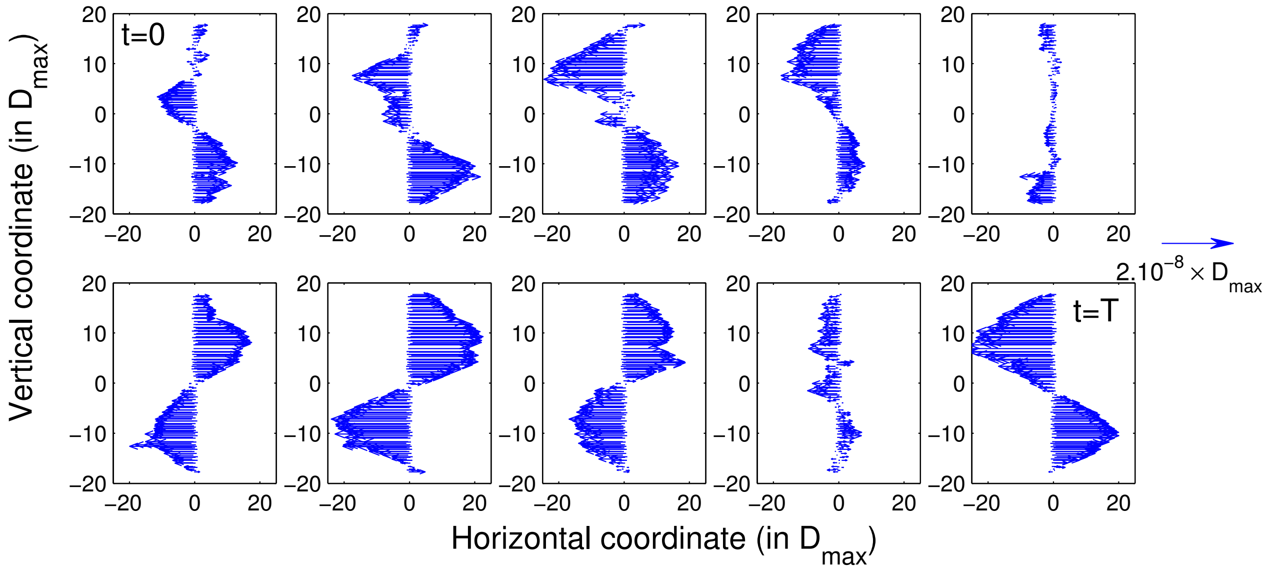


Figure 2: Snapshots of selected displacements of grains associated to an oscillation period $T$ along the radial direction. Time increases from left to right and top to bottom. The displacement scale of arrows is provided on the right of the snapshots.

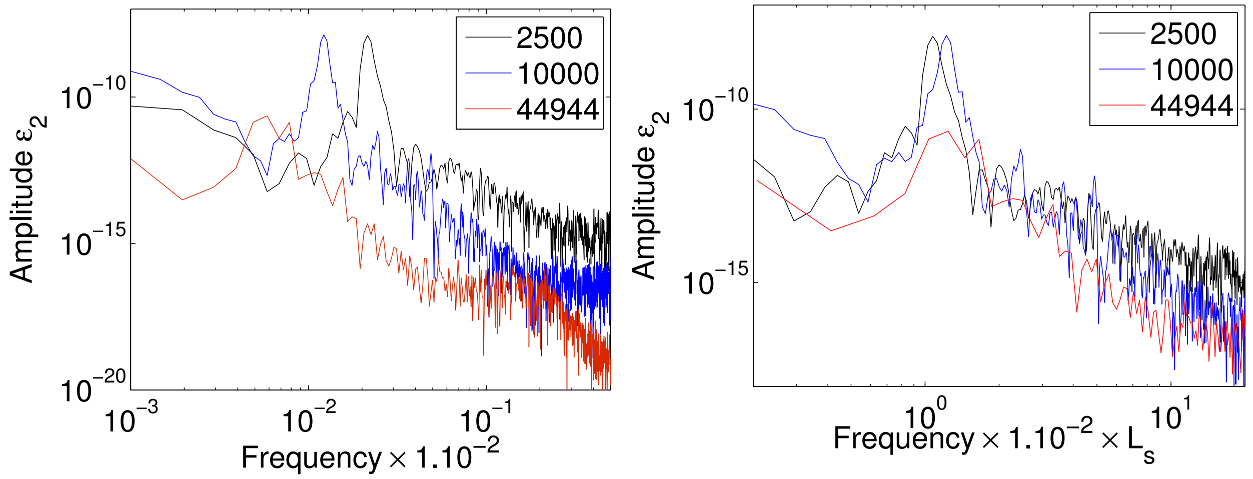


Figure 3: (Left) Fourier spectra of the radial deformation rate $\dot{\epsilon}_2$ for various sample sizes indicated in the legend (number of grains). The respective peak indicates the frequency of oscillation, that is decreasing as the sample size is increasing. (Right) Collapse analysis performed by multiplying the frequencies by $L_s$.

# 2 Collapse analyses on the shear stress rate and incremental shear strain

## 2.1 Analytical form hypothesis

The behaviour of $< x >$ with respect to the non dimensional spatial scale $l = L/D_{max}$ shown on Figure 4 and Figure 5 of the main text, where $x$ characterizes whether the shear stress rate $\dot{\tau}$ or the incremental shear deformation $\delta\gamma$, can be expressed as

$$< x > (l, \Delta) \sim l^{-\rho_x} H(l/l^*_x) \tag{3}$$

where $H(l/l^*_x) \sim const$ for $l << l^*_x$ and $H(l/l^*_x) \sim l^{\rho_x}$ for $l >> l^*_x$ [1].

We hypothesize that:

- for an infinite system, i.e. when $L_s \rightarrow +\infty : l^*_x \sim \Delta^{-\nu_x}$
- for $L_s$ finite and $\Delta \rightarrow 0 : l^*_x \sim L^{\delta_x}$ where $\delta_x$ is a fractal exponent
- for $L_s$ finite and $\Delta >> 0$, the finite size effect becomes negligible, as $l^*_x << L_s$.

A relation in agreement with these 3 hypotheses is

$$l^*_x \sim \frac{L^{\delta_x}_{sample}}{\Delta^{\nu_x} L^{\delta_x}_{sample} + C} \tag{4}$$

where $C$ is a constant.

To check this hypothesis, the collapse analyses of insets of Figure 3 and 4 are performed by doing the following change of variable

$$\begin{cases} X = l \frac{\Delta^{\nu_x} L^{\delta_x}_{sample} + C}{L^{\delta_x}_{sample}} \\ Y = < x > \left[ \frac{\Delta^{\nu_x} L^{\delta_x}_{sample} + C}{L^{\delta_x}_{sample}} \right]^{-\rho_x} \end{cases} \tag{5}$$

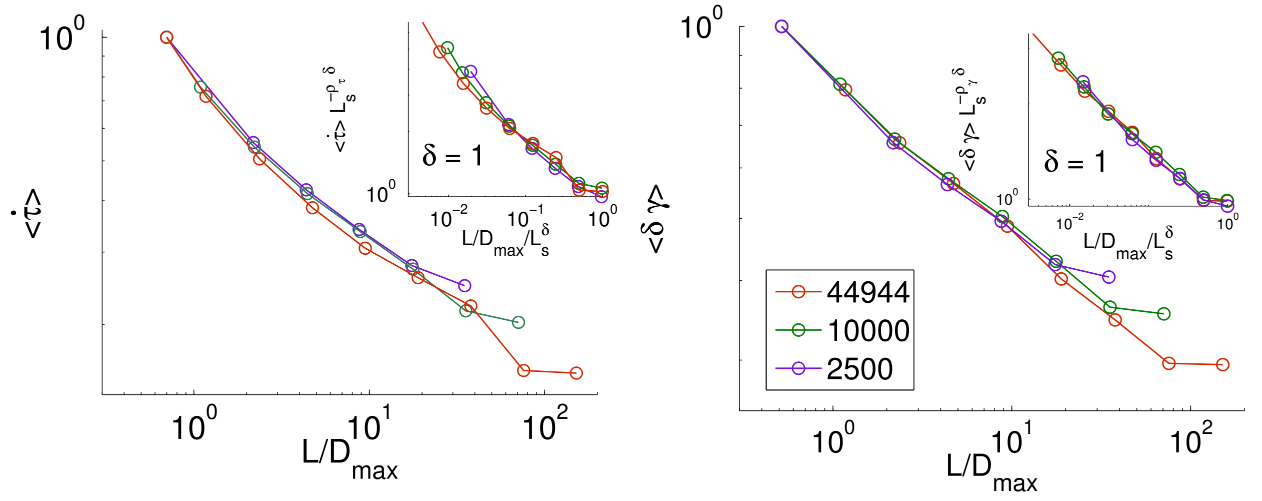


Figure 4: Multi-scale analysis performed at $\Delta = 0.005$, i.e. close to the critical point, on the (Left) shear stress rate field and (Right) incremental shear strain field, for various sample sizes indicated in the legend (number of grains). We check that $l_x^* \sim L_s^{\delta_x}$ by data collapse, shown in the insets. We find $\delta_\tau = \delta_\gamma = 1$.

## 2.2 Finite size effects

To characterize finite size effects, we perform our scaling analysis procedure close to the critical point, here at $\Delta = 0.005$, considering sample sizes of 2500, 10000 and 44944 grains loaded at constant stress rates, setting $\delta\sigma_1^{t_r} = 1.10^{-6}\sigma_3$. Figure S4 shows scalings obtained on the shear stress rate and incremental shear strain fields. For the stress field, the temporal scale considered is the wave traveling time $T$ defined in equation 1, that varies with sample size. For the strain field, the value of $\delta\epsilon_p$ needed to preserve the scaling is observed to decrease slightly with increasing sample size. We here consider $\delta\epsilon_p = 5.10^{-6}$ for 44944 grains samples, $\delta\epsilon_p = 1.10^{-5}$ for 10000 grains samples and $\delta\epsilon_p = 2.10^{-5}$ for 2500 grains samples.

Close to the critical point and on both stresses and strains, the crossover scale directly depends on sample size $L_s$. A collapse analysis shows that $l_x^* \sim L_s^{\delta_x}$, where $\delta_x = 1$.

# 3 Multi Fractal Analysis

The scale dependant heterogeneity of deformation is here examined more thoroughly by use of a multi-fractal analysis which characterizes the scaling of the moments $< x^q >$ for $0 \leq q \leq 3$. This moment analysis is a way to investigate the scale dependance of the entire distribution of $x$. Generalizing equation 4, we estimate the scaling exponents $\rho_x(q)$ and the critical exponents $\nu(q)$ by data collapse analysis for shear stresses and strains, respectively [2].

Exemples for scalings of moments $< \dot{\tau}^q >$ are plotted on Figure S5, for $q = 0.5$ and $q = 2$. Exponents $\nu_\gamma = \nu_\tau = 1.3$ are found to be constant with respect to the moment order $q$ as one would expect for a correlation length while $\rho_x(q)$ shows a curvature indicating multifractality (Figure S6) for both the stress and strain fields. By performing a quadratic fit of the form $\rho_x = a_x q^2 + b_x q + c_x$, we find $a_\tau = 0.165$ and $a_\gamma = 0.200$.

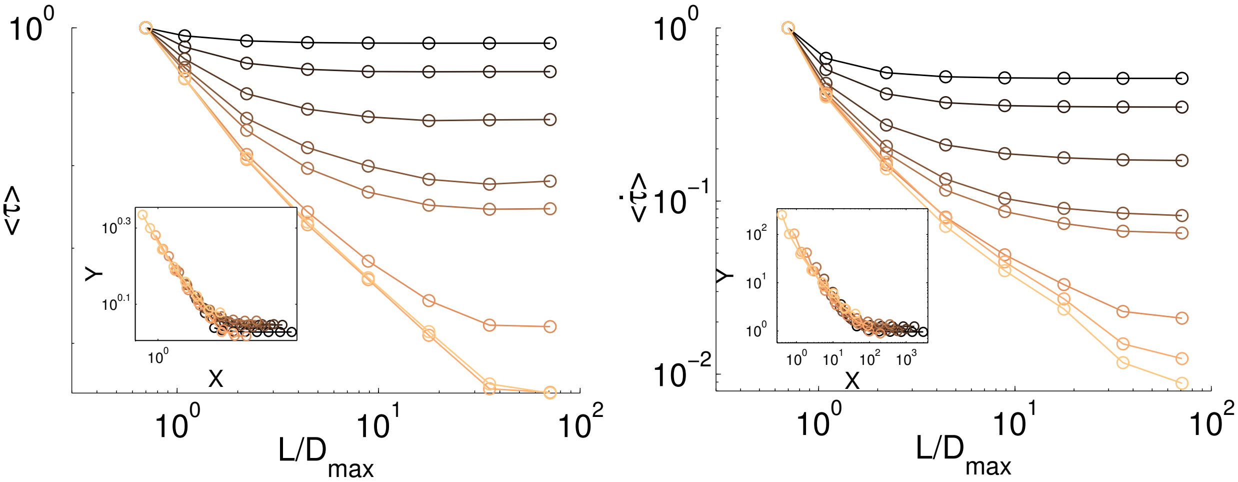


Figure 5: Multi-scale analysis performed on the shear stress field for (left) $q = 0.5$ and (right) $q = 2$. Insets show data collapse, where $X$ and $Y$ are defined in equation 5.

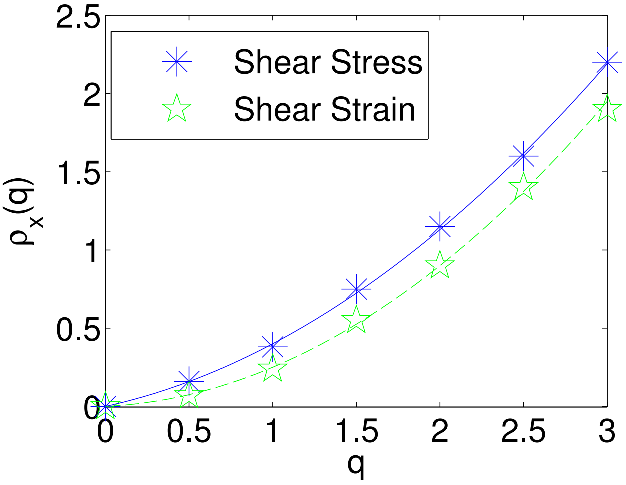


Figure 6: Values of $\rho_x$ as a function of $q$. Lines display quadratic fits of the form $a_x q^2 + b_x q + c_x$. We find $a_\tau = 0.165$, $b_\tau = 0.235$ and $c_\tau = 0$ for stresses and $a_\gamma = 0.200$, $b_\gamma = 0.05$ and $c_\gamma = 0$ for strains.

# 4 Sensitivity to increasing macroscopic loading rates

We here examine the effect of varying the macroscopic loading rate on the specific scalings evidenced on Figure 4 and Figure 5 of the main text. We here only report results obtained considering the incremental shear strain field, while the same conclusions can be drawn considering the shear stress rate field.

Figure S7(Right) shows the multi-scale analysis performed on the incremental shear strain field close to the critical point, e.g. here at $\Delta = 0.005$, considering 3 different values of macroscopic loading rate $\delta\sigma_1^{t_r}/\sigma_3$ of $1.10^{-7}$ (as considered in section 1), $1.10^{-6}$ (as considered in the main text) and $5.10^{-6}$. The value of the inertial number $I$ as a function of the normalized shear stress $\tau/\sigma_3$ is plotted on Figure S7(Left). In these configurations, regarding the values of $\delta\sigma_1^{t_r}$, initial values of $I$ range from $4.10^{-7}$ to $2.10^{-5}$. Here, as the result of averaging over simulations, the increase of $I$ as approaching the transition towards a dense flow regime reached at $\tau_c \approx 2\sigma_3$ is less brutal than the one shown on Figure 2 of the main text. This smoothing effect around $\tau_c$ is the result of the variability in the position of the onset of the transition towards the dense flow regime with respect to deviatoric stress from one simulation to another.

When considering the two configurations of $\delta\sigma_1^{t_r} = 1.10^{-7}$ and $\delta\sigma_1^{t_r} = 1.10^{-6}$, values of $I$ largely differ far from the dense flow transition but reach a similar value at $\Delta \sim 0$, which is about $I_C = 3.10^{-5}$. This means that, as soon as the loading rate is small enough, the transition to a dense flow regime, materialized by the full power law scalings undifferently observed on both configurations at $\Delta \sim 0$ on Figure S7(Right), is observed at a constant inertial number value $I_C$. At that point, the granular assembly enters in the dense flow regime. This interpretation is reinforced when looking to Figure S8, which shows the variation of $I$ as a function of $\epsilon_1$: for these two configurations and beyond the dense flow transition, the samples deform at the same velocity undependantly of the prescribed external loading.

On the reverse, when considering a larger loading rate $\delta\sigma_1^{t_r} = 5.10^{-6}$, the initial value of $I$ is of the order of $I_C$ from the beginning of the test, and is much larger than $I_C$ at the position where the dense flow transition is expected. For this configuration, a clear deviation from power law is observed at $\Delta \sim 0$ (see Figure S7(Right)), showing that no critical behaviour materialized by the divergence of the correlation length is observed at that point. We examined more thoroughly this configuration by changing both the hypothetic value of $\tau_c$ and $\delta\epsilon_w$ and found no way to observe any divergence of the correlation length at a given stage of the loading.

Thus, to conclude, we interpret the scalings reported on Figure 4 and Figure 5 of the main text to result from the particular nature of the quasi-static regime of deformation, as they are undifferently observed as soon as the value of $\delta\sigma_1^{t_r}$ is small enough, i.e. smaller than $\delta\sigma_1^{t_r} = 1.10^{-6}$, and no longer observed at larger values of $\delta\sigma_1^{t_r}$, e.g. here shown considering $\delta\sigma_1^{t_r} = 5.10^{-6}$, where the mechanical behaviour of the sample is in that case more related to a dense flow regime from the early stages of multi-axial deformation. In that case, we expect inertial effects to overcome the structures that would be inherited from stress redistributions of elastic energy in case of a slow driving load. This observation is consistent:

- with the decrease of cooperative length scales with increasing shear rate observed by [3] in glassy materials,

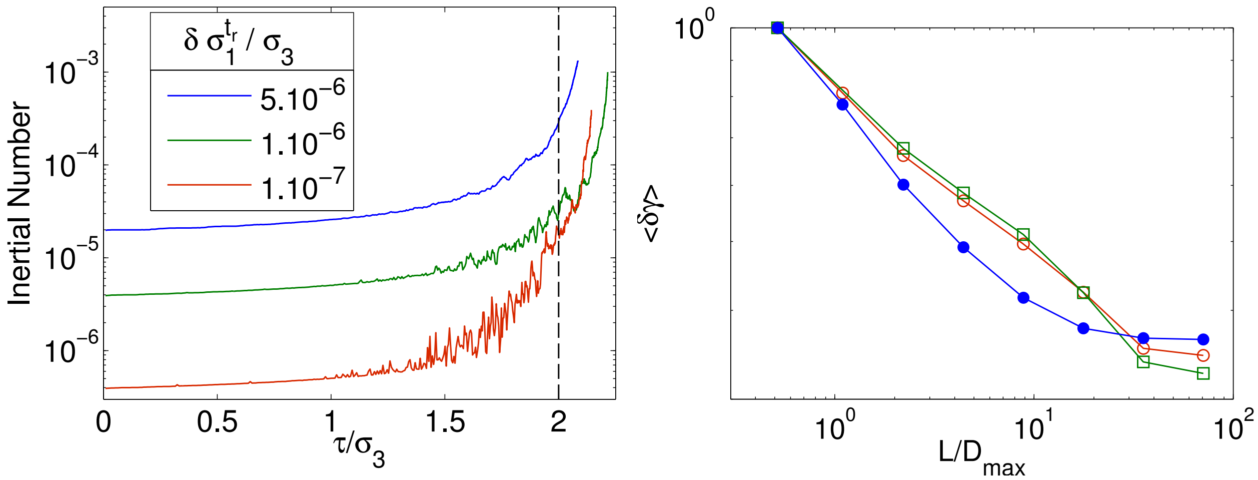


Figure 7: Effect of the loading velocity on the multi-scale properties of the incremental shear strain field. (Left) Inertial number as a function of $\tau/\sigma_3$ for various values of imposed loading rates indicated in the legend. (Right) Associated multi-scale analysis computed on the incremental shear strain field (colors correspond with (Left)) considering $\Delta = 0.005$.

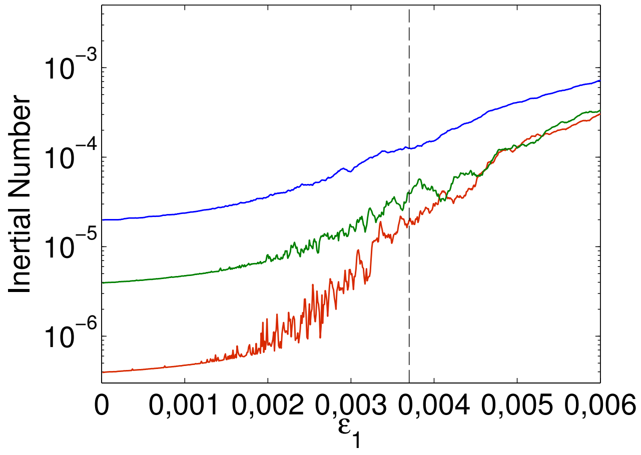


Figure 8: Inertial number as a function of $\epsilon_1$ for various values of imposed loading rates indicated in the legend of Figure 7 (colors correspond).

- with the decrease of velocity fluctuations with increasing values of inertial number $I$ reported in [4] for frictional granular materials submitted to various loading configurations.

# References


[1] GIRARD, L., AMITRANO, D. and WEISS, J., Failure as a critical phenomenon in a progressive damage model. Journal of Statistical Mechanics: Theory and Experiment, J. Stat. Mech. (2010) P01013.

[2] MARSAN, D., STERN, H., LINDSAY, R. and WEISS, J., Scale Dependance and Localization of the Deformation of Arctic Sea Ice, Phys. Rev. Lett. **93** (2004) 178501.

[3] TSAMADOS, M., Plasticity and dynamical heterogeneity in driven glassy materials, Eur. Phys. J. E. **32** (2010) 165–181.

[4] GDR MiDi, On dense granular flows, Eur. Phys. J. E. **14** (2004) 341-365.
